# Supplementary material for: Active Classification of Moving Targets with Learned Control Policies
Source: arXiv:2212.03068 source file (2023-09-27)
Supplement: Supplementary file 1 [file AppendixC.tex]

\section{First-order vs. drone dynamics} \label{sec:appendixC}
We compare the performance of our learned policy under first order dynamics versus its performance under drone dynamics (Appendix \ref{sec:appendixD}) for a varying number of targets. All other test conditions (see Section \ref{sec:results}) are maintained. Even when the policy has been trained with first order dynamics, Figure \ref{fig:dynamics_change} shows there is no significant difference of performance between both situations. We speculate that the small difference in performance is due to the low-level controller smoothing the behavior and trajectories of the drone.

\begin{figure}[!h]
    \centering
    \includegraphics[width=0.5\textwidth]{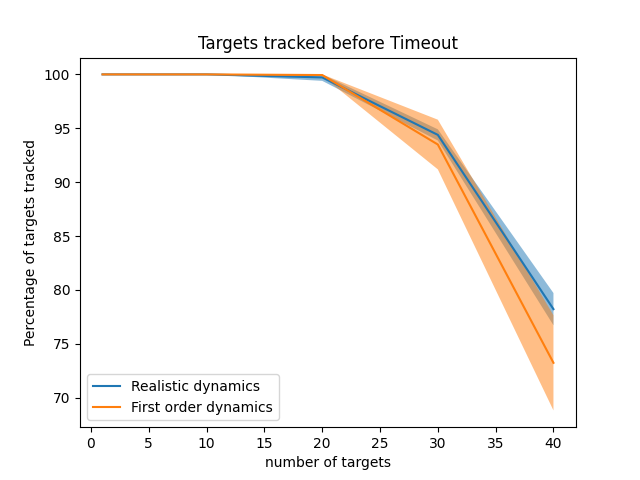}
    %\vspace{-13mm}
    \caption{\footnotesize{Performance comparison of our method under first-order and realistic dynamics. }}
    \label{fig:dynamics_change}
\end{figure}

% First order dynamics vs. Drone dynamics. --check

% Not realistic but rather drone dynamics. --check

% Text very unclear, we re just comparing the number of methods for a varying number of targets

% Missing comment about why the blue one looks better than the orange one. Not sig different but still we need a comment on why it is different. Why is it different when the original is worse. -- check

% Compute trajectories and check -- check

% Sentece we speculate that difference in performance smoothes the behavior and trajectories of the drone   %%%%% HIGH PRIORITY. check
