# Supplementary material for: Active Classification of Moving Targets with Learned Control Policies
Source: arXiv:2212.03068 source file (2023-09-27)
Supplement: Supplementary file 2 [file AppendixD.tex]

\section{Robot model and cost function}\label{sec:appendixD}
\subsection{Robot model}
In this work, we use the same drone model and specifications for the Parrot Bebop2 SDK as in~\cite{Zhu2019}. According to the Parrot Bebop2 SDK, the control inputs to the quadrotor are given by $\vu=[\phi_c,\theta_c,v_{z_c},\dot{\psi}_c]\in\mathbb{R}^4$, where $\phi_c$ and $\theta_c$ are the desired roll and pitch angles, $v_{z_c}$ is the desired linear velocity in the z-axis and $\dot{\psi}_c$ is the yaw rate. To simulate the drone dynamics, we use the full state of the drone (position, velocity and attitude) denoted by $\vx^{full}_t=[q_x,q_y,q_z,v_x,v_y,v_z,\phi_t,\theta_t, \psi_t] \in\mathbb{R}^9$. We use a first order low-pass Euler approximation of the quadrotor dynamics~\cite{Zhu2019}, where the dynamics of the state velocity vector are:

\begin{equation}
    \left\{
    \begin{array}{lll}
        \begin{bmatrix}
        \dot{v}_x\\
        \dot{v}_y
        \end{bmatrix} = 
        Rot_Z(\psi)\begin{bmatrix}
        \tan\theta\\
        -\tan\phi
        \end{bmatrix}g-
        k_D\begin{bmatrix}
        v_x\\
        v_y
        \end{bmatrix},
        \\[5mm]
        \dot{v}_z = \frac{1}{\tau_{v_z}}(k_{v_z}v_{z_c}-v_z),
    \end{array}
    \right.
\end{equation}

where $g=9.81 m/s^2$ is the earth's gravity, $Rot_Z(\psi) \in SO(2)$ is the rotation matrix along the drone's local z-axis, $k_D$ is the drag coefficient, $k_{v_z}$ and $\tau_{v_z}$ are the gain and time constant of vertical velocity.
The attitute dynamics of the quadrotor are:
 \begin{equation}
     \dot{\phi}= \frac{1}{\tau_\phi}(\phi_c-\phi),\hspace{5mm} \dot{\theta}=\frac{1}{\tau_\theta}(\theta_c-\theta),\hspace{5mm} \dot{\psi}=\dot{\psi_c}
 \end{equation}
 
 %where $k_\phi,k_\theta$ and $\tau_\phi,\tau_\theta$ are the gains and time constant of roll and pitch angles respectively.
 where $\tau_\phi,\tau_\theta$ are the time constants of roll and pitch angles respectively.
 
 In this work, the height of the drone is fixed at $q_z=2.4m$ so that it can fly over targets. Due to the camera heading $\psi^0$ being independent from the drone's, we fix the drone's yaw angle to zero. Consequently, $v_{z_c} = \dot{\psi}_c =0$.

% \subsection{Cost Function}
% The cost functions $J^k(\vx^k,\vu^k), k= 0,1,\dots,N-1$ and $J^N(\vx^N,\va)$, where $\va = [\Delta q_{x'}, \Delta q_{y'}, \Delta\psi]$ is the recommended viewpoint at time step $t$ in the camera's local reference, are defined in the following. 

% \textbf{Goal navigation}~~~~We minimize the displacement between the trajectory's terminal position and the robot's goal location, and define a terminal cost,
% \begin{equation}
%     J^N(\vx^N, \va) = w^N\frac{\norm{\vq^N-\vg_{a}}}{\norm{\vq^0-\vg_{a}}},
% \end{equation}
% where $\vq$ denotes position in the x-y plane, $\vg_{a} = \vq^0 + R_Z(\psi^0)[\Delta q_{x'}, \Delta q_{y'}]^T$ denotes the recommended viewpoint position in global reference, and $w^N \in \R^+$ is a tuning weight coefficient. 

% \textbf{Control input cost}~~~~The stage cost is used to minimize the control input, 
% \begin{equation}
%     J^k(\vx^k,\vu^k) = J_{u}^k(\vu^k) = w_{u}\norm{\vu^k},
% \end{equation}
% where $w_{u} \in \R^+$ is a tuning weight coefficient. 

%the commanded angular velocity around the z-body axis.
%We consider the model of the Parrot Bebop2 SDK
