# Supplementary material for: Active Classification of Moving Targets with Learned Control Policies
Source: arXiv:2212.03068 source file (2023-09-27)
Supplement: Supplementary file 3 [file AppendixE.tex]

\section{Additional Results}
%\vspace{-3mm}
\begin{figure*}[t!] 
        \captionsetup[subfigure]{position=b}
        \begin{subfigure}{0.32\textwidth}
                \includegraphics[width=\textwidth]{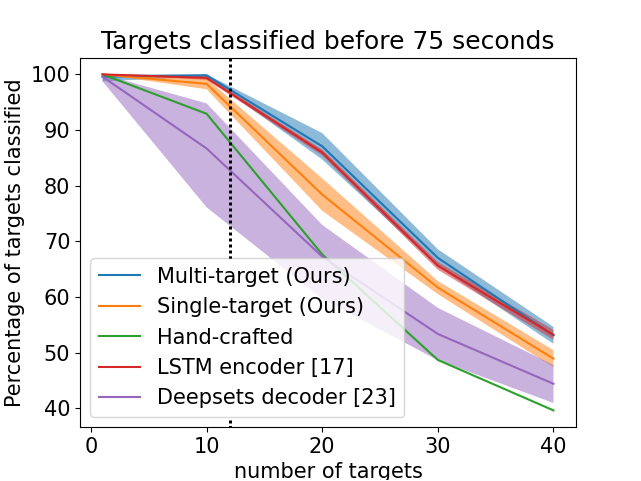}
        %\vspace{-5mm}
        \caption{\footnotesize{Constant velocity}\label{fig:additionalScalability}}
        \end{subfigure}
        % \hfill
        ~
        \captionsetup[subfigure]{position=b}
        \begin{subfigure}{0.32\textwidth}
                \includegraphics[width=\textwidth]{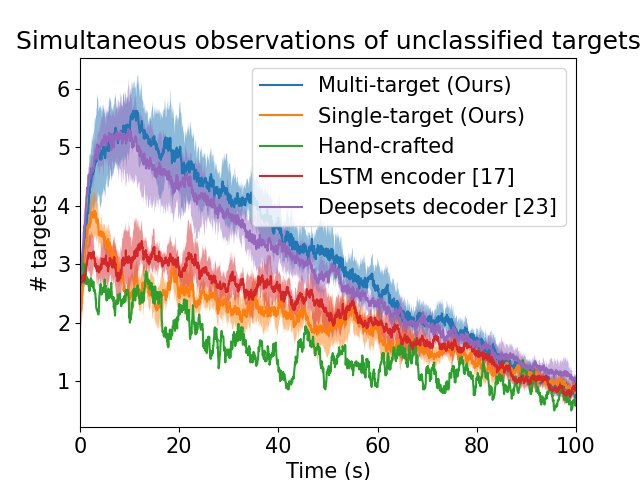}
        %\vspace{-5mm}
        \caption{\footnotesize{Constant velocity}\label{fig:additionalSimultaneous_observation}}
        \end{subfigure}
        % \hfill
        ~
        \captionsetup[subfigure]{position=b}
        \begin{subfigure}{0.32\textwidth}
                \includegraphics[width=\textwidth]{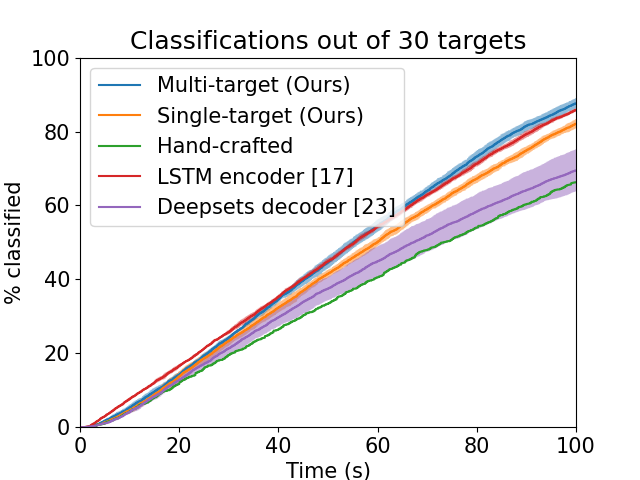}
        %\vspace{-5mm}
        \caption{\footnotesize{Constant velocity}\label{fig:additionalClassificationspeed}}
        \end{subfigure}
        % \hfill
        ~
        % \captionsetup[subfigure]{position=b}
        % \begin{subfigure}{0.32\textwidth}
        %         \includegraphics[width=\textwidth]{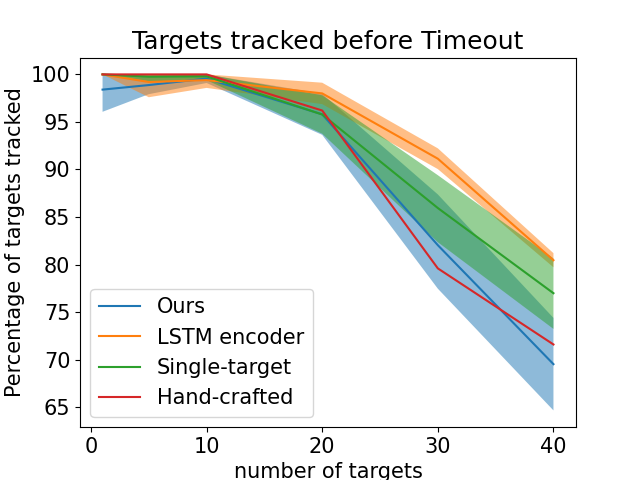}
        % \vspace{-5mm}
        % \caption{\footnotesize{Static}\label{fig:classificationspeed}}
        % \end{subfigure}
        % % \hfill
        % ~
        % \captionsetup[subfigure]{position=b}
        % \begin{subfigure}{0.32\textwidth}
        %         \includegraphics[width=\textwidth]{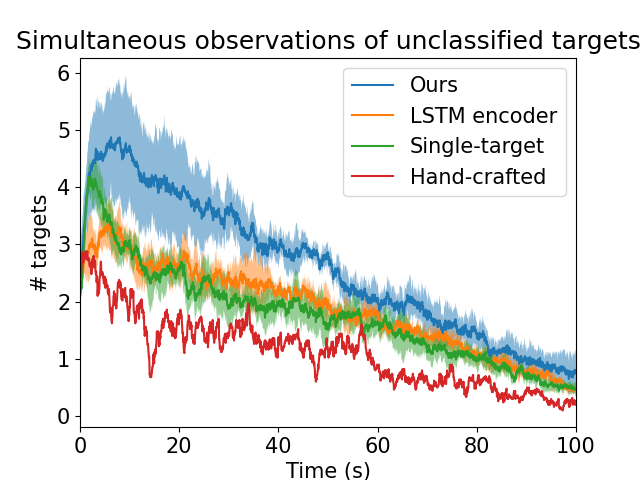}
        % \vspace{-5mm}
        % \caption{\footnotesize{Static}\label{fig:classificationspeed}}
        % \end{subfigure}
        % % \hfill
        % ~
        % \captionsetup[subfigure]{position=b}
        % \begin{subfigure}{0.32\textwidth}
        %         \includegraphics[width=\textwidth]{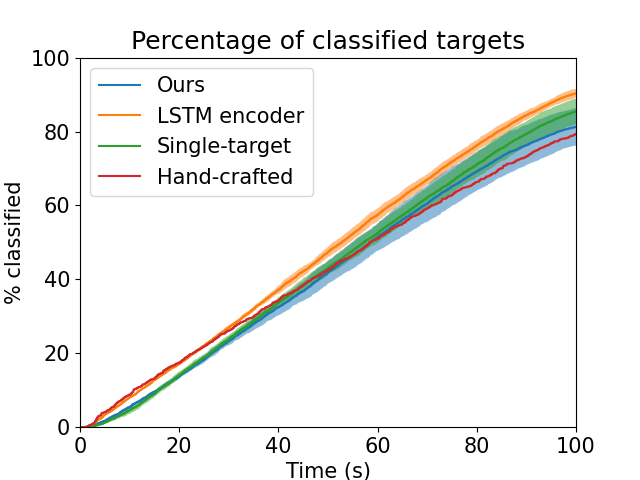}
        % \vspace{-5mm}
        % \caption{\footnotesize{Static}\label{fig:classificationspeed}}
        % \end{subfigure}
        % \hfill
        % ~
        % \captionsetup[subfigure]{position=b}
        % \begin{subfigure}{0.50\textwidth}
        %         \includegraphics[width=\textwidth]{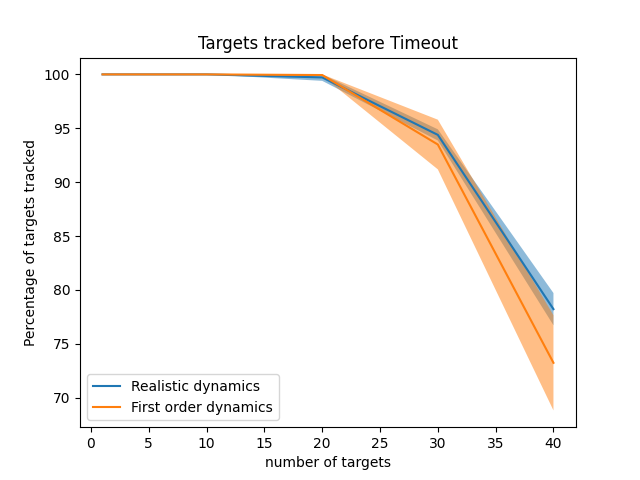}
        % \vspace{-5mm}
        % \caption{\footnotesize{}\label{fig:dynamics_change}}
        % \end{subfigure}
        % % \hfill

        %\vspace{-5mm}
        \caption{\footnotesize{Comparison of our method and the baselines in environments where targets follow constant velocity dynamics. \textbf{(a)}~Comparison of the percentage of targets classified before timeout in environments with 1 to 40 targets.~\textbf{(b)}~Evolution of simultaneous observations along the episode in environments of 30 targets.~\textbf{(c)}~Classification speed in environments of 30 targets.%~\textbf{d)}~Performance comparison of the policy under first order and realistic dynamics.
        }} \label{fig:additionalResults}
\end{figure*}

\subsection{Performance under different target dynamics}
%\vspace{-3mm}
We further evaluate all methods in environments with varying number of targets following constant velocity dynamics. All other test conditions are maintained (see Section \ref{sec:results}). In Figure \ref{fig:additionalScalability}, we report the percentage of targets that each method has been able to classify in this setting. Similar to the results shown in Section \ref{sec:results}, our method clearly outperforms both the \textit{Hand-crafted} and \textit{Single-target} baselines in environments with more than ten targets. However, the performance of our learned policy is not significantly higher in comparison with the \textit{LSTM encoder} baseline, despite our method consistently observing more unclassified targets simultaneously over time as shown in Figure \ref{fig:additionalSimultaneous_observation}. Our method's architecture learns to prioritise quantity over quality of observations over the set of unclassified targets. Instead, the \textit{LSTM encoder} baseline, by definition (see its description in Section \ref{sec:results}), prioritises and retains more information of unclassified targets according to their proximity. This results in less amount but more informative target observations per timestep. 

%Our architecture is able to account for all target's available information at the same time. This means that it is able to learn strategies that are likely to infer target priority and go towards viewpoints allowing simultaneous observations of multiple unclassified targets. Instead, the \textit{LSTM encoder} baseline requires each target to be fed sequentially, retaining more information of the last input targets. Due to targets in a sequence being ordered according to proximity and being already identified, the learned policy from the baseline will effectively prioritise close unclassified targets. This will result in a poor number of clse

%Apart from being trained under the same conditions...

%Our architecture is able to account for all target's available information at the same time. This means that it is able to learn strategies that are likely to prioritise to go towards viewpoints allowing simultaneous observations of multiple unclassified targets. 

%% Give context to results shown using RSS

%% Make clear that the training environment is dynamic which do es not happen anymore

%% Plots
 % put the plots in the same scale
 %% Static explanation why static performs worse even though simul obs are higher than others.
 % prioritising quantity over quality.
 
 % Look into this environment with cte vel and looks similar to the one in the paper.

%\vspace{-3mm}
%\vspace{-8mm}
\subsection{Policy behavior}
%\textbf{Policy behavior}~~~~
%\vspace{-3mm}
\begin{figure*}[ht]
        \centering
        \captionsetup[subfigure]{position=b}
        \begin{subfigure}{0.43\textwidth}
                \includegraphics[width=\textwidth]{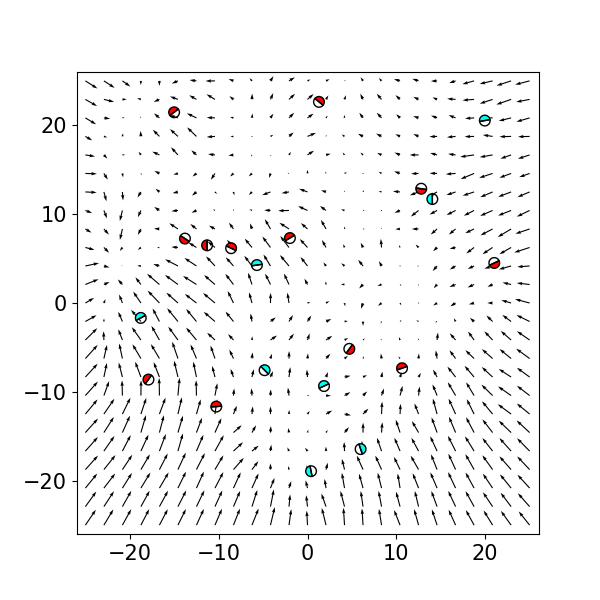}
        %\vspace{-5mm}
        \caption{\footnotesize{}\label{fig:qualitative_position}}
        \end{subfigure}
        % \hfill
        ~
        \captionsetup[subfigure]{position=b}
        \begin{subfigure}{0.43\textwidth}
                \includegraphics[width=\textwidth]{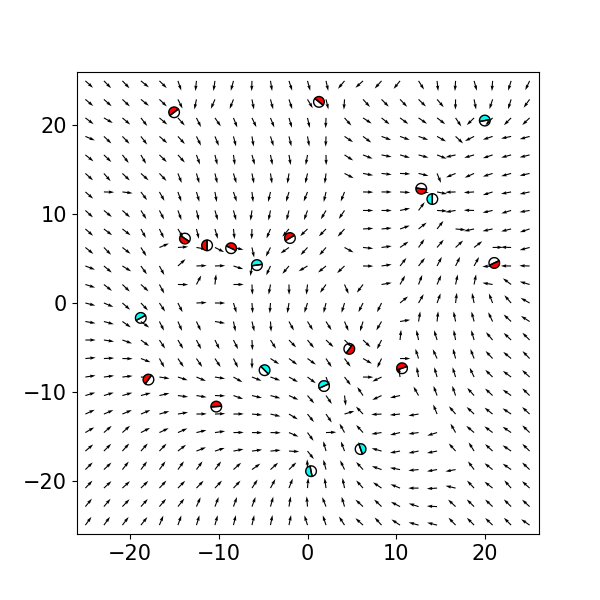}
        %\vspace{-5mm}
        \caption{\footnotesize{}\label{fig:qualitative_orientation}}
        \end{subfigure}
        % \hfill
        %\vspace{-5mm}
        \caption{\footnotesize{Given a set of targets we plot \textbf{(a)} vectors representing the recommended viewpoint given by the learned policy at each position of the environment and \textbf{(b)} the orientation to which the learned policy turns the camera heading.}} \label{fig:qualitative}
\end{figure*}
We present additional qualitative and intuitive results of the learned policy behavior. Given a set of twenty targets, no previous information over them, and a position of the drone, we plot the recommended viewpoint position to where the learned policy guides the drone (Figure \ref{fig:qualitative_position}). We also plot the orientation to which the learned policy would stir the camera heading if given enough time (Figure \ref{fig:qualitative_orientation}). As expected, the learned policy guides the drone towards positions from where the drone can observe multiple targets, and turns the camera towards orientations which allow it to obtain multiple target observations.

%Figure \ref{fig:qualitative_position} shows the position the drone is guided 
%\vspace{-2.5mm}

%% Give context to results shown using

%% Make clear that the training environment is dynamic which do es not happen anymore

%% Plots
 % put the plots in the same scale
 %% Static explanation why static performs worse even though simul obs are higher than others.
 % prioritising quantity over quality.
 
 % Look into this environment with cte vel and looks similar to the one in the paper.
