# Supplementary material for: Active Classification of Moving Targets with Learned Control Policies
Source: arXiv:2212.03068 source file (2023-09-27)
Supplement: Supplementary file 4 [file AppendixG.tex]

\section{Intuition behind learning target relationships through self-attention}\label{appendixG}

\begin{figure}[ht]
    \centering
    \includegraphics[width=0.55\textwidth]{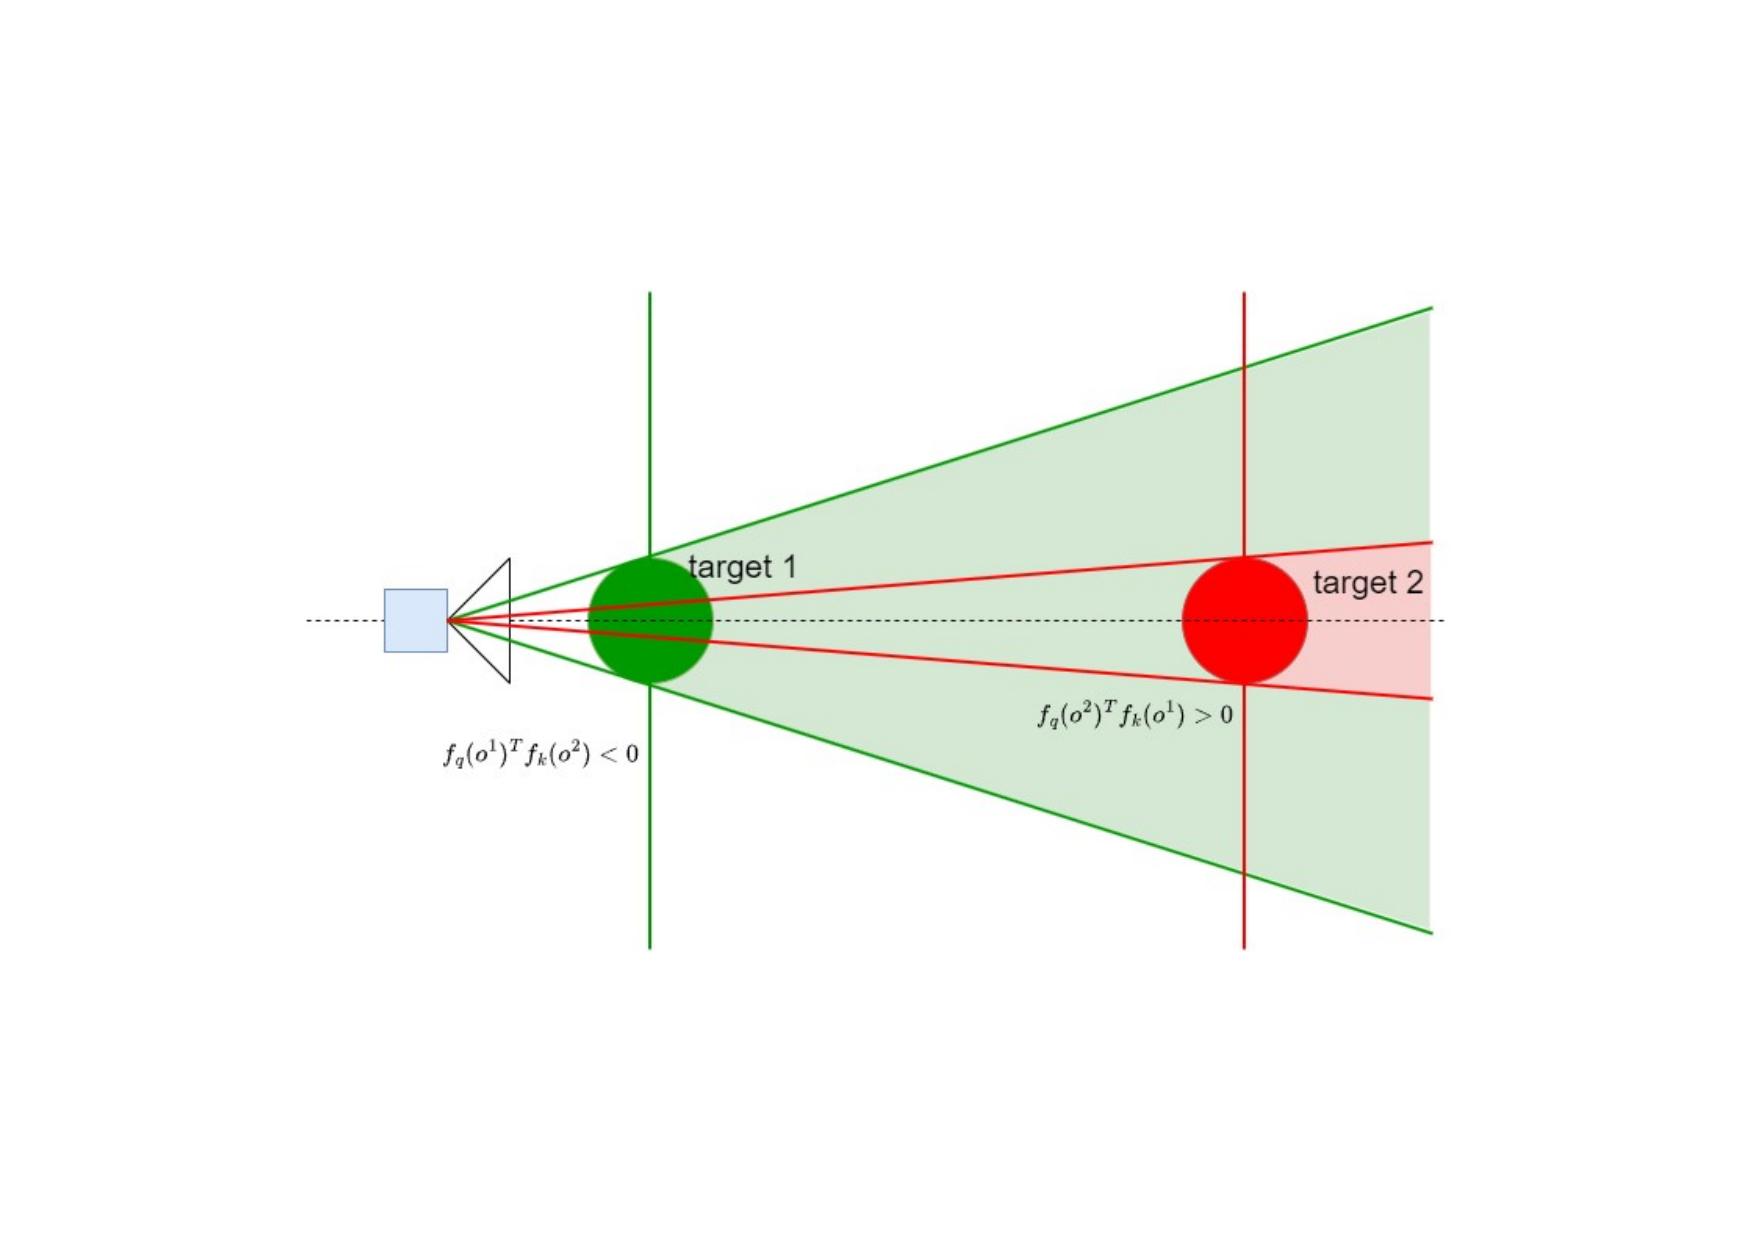}
    %\vspace{-4mm}
    \caption{\footnotesize{Example of asymmetric relations between two targets. Target 2 belongs to the subspace occluded by target 1. Therefore, target 2's latent encoding is modified by the presence of target 1. In this example the effect of target 2 on target 1's encoding is much lower.}}
    \label{fig:example_occlusions}
\end{figure}

\newcont{The main motivation behind using attention layers is their capability to learn asymmetric relationships among targets. This allows occluding targets to modify the resulting encoding of occluded targets, but not the other way around. In the handcrafted sketched example attached to the comment, the learned affine transformation $f_k(\mathbf{o}^i) \coloneqq f(\vo^i;\mathbf{W}_{k}^1)$ has learned to associate each target i to 3 half-spaces, the union of which represents the subspace occluded by it. Instead, $f_q(\mathbf{o}^j) \coloneqq f(\vo^j;\mathbf{W}_{v}^1)$ has learned a latent representation of target j that, in combination with $f_k(\mathbf{o}^i)$, e.g. $f_q(\mathbf{o}^j)^Tf_k(\mathbf{o}^i)$, allows to identify whether target j is occluded by target i. 

Thus, in this example, only target 2 is occluded by target 1. This results in the self-attention weights $\lambda_{1,2}, \lambda_{2,1}$ being different and $\lambda_{2,1}>\lambda_{1,2}$.}
