# Supplementary material for: Active Classification of Moving Targets with Learned Control Policies
Source: arXiv:2212.03068 source file (2023-09-27)
Supplement: Supplementary file 5 [file AppendixF.tex]

\section{Extension to more realistic settings}\label{appendixF}
\subsection{Higher-fidelity perception}\label{F_perception}
