# Supplementary material for: Active Classification of Moving Targets with Learned Control Policies
Source: arXiv:2212.03068 source file (2023-09-27)
Supplement: Supplementary file 6 [file POMDP_formulation.tex]

%\subsection{Reinforcement Learning}\label{sec:appendixA}
\section{POMDP Formulation}

\subsection{Action Space $\cA$}
Every time step, the drone leverages the information it has available and chooses the next viewpoint in its neighborhood to move towards, expressed in terms of its camera local reference frame. In practice, this translates into choosing:
\begin{equation}
\begin{split}
    \va_t := [\Delta q_{x',t}, \Delta q_{y',t}, \Delta\psi_{t}]\\
\end{split}
\end{equation}
where $x',y'$ represent the $x$ and $y$-axis in the camera's local reference, and $\Delta q_{i,t}$, $\forall i\in\{x',y'\}$ are confined to a neighborhood of the current drone's pose: $\Delta q_{x',t},\Delta q_{y',t}\in[-\Delta q^{max},\Delta q^{max}]$, where $\Delta q^{max}$ denotes the maximum distance along each local axis that the drone can reach within one second at constant velocity. This also applies for the camera heading $\psi^0$. 
